# Supplementary material for: Dynamical-System Model Predicts When Social Learners Impair Collective Performance
Source: arXiv:2104.00770 ancillary file (2021-08-20)
Supplement: Supplementary file 1 [file SI.pdf]

# Supplementary Information for Dynamical-System Model Predicts When Social Learners Impair Collective Performance

Vicky Chuqiao Yang, Mirta Galesic, Harvey McGuinness, Ani Harutyunyan

## Contents

|          |                                                         |          |
|----------|---------------------------------------------------------|----------|
| <b>1</b> | <b>Derivation of the mathematical model</b>             | <b>1</b> |
| <b>2</b> | <b>Analyzing the fixed points</b>                       | <b>3</b> |
| <b>3</b> | <b>Analytical results for general <math>f(x)</math></b> | <b>3</b> |
| <b>4</b> | <b>Results for <math>\alpha &lt; 1</math></b>           | <b>4</b> |
| <b>5</b> | <b>Model extensions</b>                                 | <b>4</b> |
| 5.1      | Spectrum extension                                      | 4        |
| 5.2      | Spatial extension                                       | 5        |
| 5.3      | Noise extension                                         | 6        |
| 5.4      | Opinion strength extension                              | 6        |
| <b>6</b> | <b>Code availability</b>                                | <b>7</b> |

## 1 Derivation of the mathematical model

We develop a dynamical-system model of collective decision making in a binary choice task to investigate the interplay of the proportion of individual vs. social learners, the relative merit of two options for individual learners, and the shape of conformity response for social learners.

First, individuals can use different cognitive strategies when choosing an option. They may prefer to ground their decisions primarily in their own exploration of the merit of different options, such as evidence or personal values (individual learners), or they may prefer to follow choices of others around them (social learners) for informational or conformist reasons [1]. The cognitive strategies an individual will use can depend on contextual differences, including how easy it is to learn on one's own about the merit of different options, availability of suitable models, and cultural differences regarding the value of conformity [2, 3].

Second, tasks that involve a choice between options can differ regarding the amount of evidence in favor of one option or the other. Real-world contexts are often characterized by layers of uncertainty that make evidence for different options unclear [4, 5]. Examples are tasks in political, financial, health, and environmental domains, in particular in novel, uncertain, and evolving contexts [6–9]. In these situations, different options can be perceived as having quite similar merits, and the processes of social influence can be critical in determining the winning option [10–13].

Third, the likelihood of an individual adopting an option generally increases with the frequency of others adopting it in the overall population [14]. However, this relationship, which we refer to as the *conformity function*, can take many functional forms. It can be linear, whereby the likelihood of an option being chosen equals its frequency in the population; S-shaped, the likelihood of adoption is higher than option frequency; or inverse-S-shaped, whereby the frequency is lower than the frequency of that option in

the population [15]. The exact shape might depend on factors such as group size [16] and on whether individuals seek to adapt to their nonsocial environments (informational conformity) or fit into their social environments (normative conformity) [1]. Normative conformity is typically associated with an S-shaped conformity response function, and informational conformity is typically associated with a linear or inverse-S-shaped function.

The formulation of the transition rates,  $P_{YX}$  and  $P_{XY}$  in Eq. 1 of the main text is as follows. First, the mixture of cognitive strategies is incorporated as a population variable—the population consists of portion  $s$  social learners, and  $1 - s$  individual learners. We assume individuals do not change their cognitive strategies for a given issue.

Second, we consider individual learners to change their opinion about the options based on independent consideration of evidence and values. We express the merit of opinion  $X$  relative to  $Y$ , denoted as  $m$ , to be the transition rate of an individual switching from  $Y$  to  $X$ ,  $P_{YX}^{(i)} = m$ . By symmetry,  $P_{XY}^{(i)} = 1 - m$ .

Third, we consider social learners' behaviors to be affected by conformity only. The transition rate for social learners from  $Y$  to  $X$  is an increasing function of the observed frequency of option  $X$  in the whole population ( $x$ ). By construction,  $x = (1 - s)x_i + sx_s$ . We define  $P_{YX}^{(s)} = f(x)$ , where  $f(x)$  is the frequency-dependent conformity response function (or conformity function later in text). According to reviews of empirical evidence [15, 17, 18], a realistic function is an monotonic increasing function symmetric about (0.5, 0.5), with alternating convexity in the upper and lower parts.

A particular functional form satisfying these conditions, which we will use for most of our following analysis is,

$$f(x) = \begin{cases} (2x)^\alpha / 2, & 0 \leq x \leq 0.5, \\ 1 - (2(1 - x))^\alpha / 2, & 0.5 \leq x \leq 1. \end{cases} \quad (\text{S1})$$

This function is parameterized by one parameter,  $\alpha$ , varying which allows for all convexities of the conformity functions observed in the literature. A plot of this function with various  $\alpha$  values is shown in Fig. 1(B) of the main text. Parameter  $\alpha > 1$  leads to S-shaped functions,  $\alpha < 1$  leads to inverse-S-shaped functions, and  $\alpha = 1$  denotes a linear response.

After accounting for the transition rates, the governing equations for social and individual learners in Eq. 1 of the main text becomes,

$$\frac{dx_i}{dt} = m(1 - x_i) - (1 - m)x_i, \quad (\text{S2})$$

$$\frac{dx_s}{dt} = f(x)(1 - x_s) - f(1 - x)x_s. \quad (\text{S3})$$

Simplifying Eqs. S2 and S3, we have

$$\frac{dx_i}{dt} = m - x_i, \quad (\text{S4})$$

$$\frac{dx_s}{dt} = f((1 - s)x_i + sx_s) - x_s. \quad (\text{S5})$$

We investigate in what conditions is the high-merit option preferred by the majority, in other words, if  $m > 0.5$ ,  $x > 0.5$  and if  $m < 0.5$ ,  $x < 0.5$ .

## 2 Analyzing the fixed points

We analyze the dynamical system's fixed points and their stability according to methods outlines in [19]. We find the fixed points by solving for  $x_i$  and  $x_s$  such that  $dx_i/dt = dx_s/dt = 0$  in Eqs. S4 and S5. The solutions are denoted as  $x_i^*$  and  $x_s^*$  respectively. Note that the term fixed points (terminology common in applied mathematics) for continuous-time dynamical systems is equivalent to equilibria in other fields (such as economics). Stable fixed points are equivalent to stable equilibria, and unstable fixed points are equivalent to unstable equilibria. In Eq. S4, it is obvious that  $x_i^* = m$ . We then solve for  $x_s^*$ . In the results presented in Fig. 2, which uses the functional form of  $f(x)$  in Eq. S1, we solve for  $x_s^*$  computationally using the Python 3 programming language. The fixed points of  $x$ , the proportion of individuals favoring  $X$ ,  $x^*$ , is then computed using its definition,  $x^* = sx_s^* + (1-s)x_i^*$ .

We then analyze the stability of the fixed points by computing the Jacobian matrices of the dynamical system (Eqs. S4 and S5) at these fixed points, and solving for the eigenvalues of these Jacobian matrices. Stable fixed points are characterized by both eigenvalues being negative, and unstable ones are characterized by at least one positive eigenvalue. The fixed points' stability shown in Fig. 2 is obtained by computing the eigenvalues of the Jacobian matrices using the Python 3 programming language.

## 3 Analytical results for general $f(x)$

Here we derive analytical predictions of our model without functional form assumptions of  $f(x)$ . We consider general increasing  $f(x)$  symmetrical about the point (0.5, 0.5). The functional form given in Eq. S1, and subsequently in Fig. 1(B), are all special cases of this general consideration. Here we derive analytical predictions of the expression of the critical transition point,  $s_c$ , under the condition of  $X$  and  $Y$  having equal merit,  $m = 0.5$ .

The point  $x_i = x_s = 0.5$  is a fixed point of the dynamical system for all  $s$  values when  $m = 0.5$ . This can be verified by plugging these values in Eqs. S4 and S5 and show the right-hand-side of both equations are 0. Note that the symmetry condition for  $f(x)$  requires  $f(0.5) = 0.5$ . Because the critical transition in  $s$  occurs when this fixed point changes stability [19], we analyze its stability by computing the Jacobian matrix of the dynamical system and it is

$$J(x_i, x_s) = \begin{pmatrix} -1 & 0 \\ f'((1-s)x_i + sx_s)(1-s) & f'((1-s)x_i + sx_s)s - 1 \end{pmatrix} \quad (\text{S6})$$

where  $f'(x_0)$  is the derivative of  $f(x)$  with respect to  $x$  evaluated at  $x_0$ . Plugging  $x_i = x_s = 0.5$  in Eq. S6, we solve for the eigenvalues of the Jacobian matrix. The two eigenvalues are  $\lambda_1 = -1$  and  $\lambda_2 = f'(0.5)s - 1$ . Since  $\lambda_1 < 0$ , the stability of the fixed point depends on the sign of  $\lambda_2$ . If  $\lambda_2 < 0$ , then  $(x_i, x_s) = (0.5, 0.5)$  is stable, and if  $\lambda_2 > 0$ , it is unstable. Solving for  $\lambda_2 = 0$ , we find the solution of this critical point is

$$s_c = \frac{1}{f'(0.5)}. \quad (\text{S7})$$

When  $s < s_c$ , (0.5, 0.5) is stable, and the system has one fixed point. When  $s > s_c$ , (0.5, 0.5) is unstable, and the system has bi-stable states. Equation S7 also shows that  $r_c$  has a solution between 0 and 1 only when  $f'(0.5) > 1$ . This predicts the bi-stable state exists only when  $f'(0.5) > 1$ . This also explains why the bi-stable state does not appear in the  $\alpha \leq 1$  case.

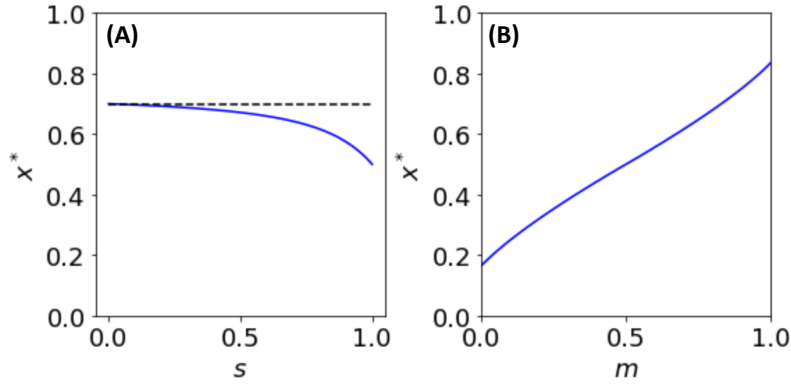

**Figure S1.** Fixed points for the proportion of individuals favoring option  $X$ ,  $x^*$  when  $\alpha = 0.8$ . (A) as a function of  $s$ , with  $m = 0.7$  (dashed line) (B) as a function of  $m$ , with  $s = 0.8$ .

## 4 Results for $\alpha < 1$

We analyze the fixed points for the case of  $\alpha < 1$  when using the functional form of  $f(x)$  in Eq. S1. The system has one fixed point through all parameters, with some examples shown in Fig. S1.  $x^*$  increases smoothly with  $m$ . When  $s = 1$ ,  $x^* = 0.5$  and when  $s = 0$ ,  $x^* = m$ .

## 5 Model extensions

### 5.1 Spectrum extension

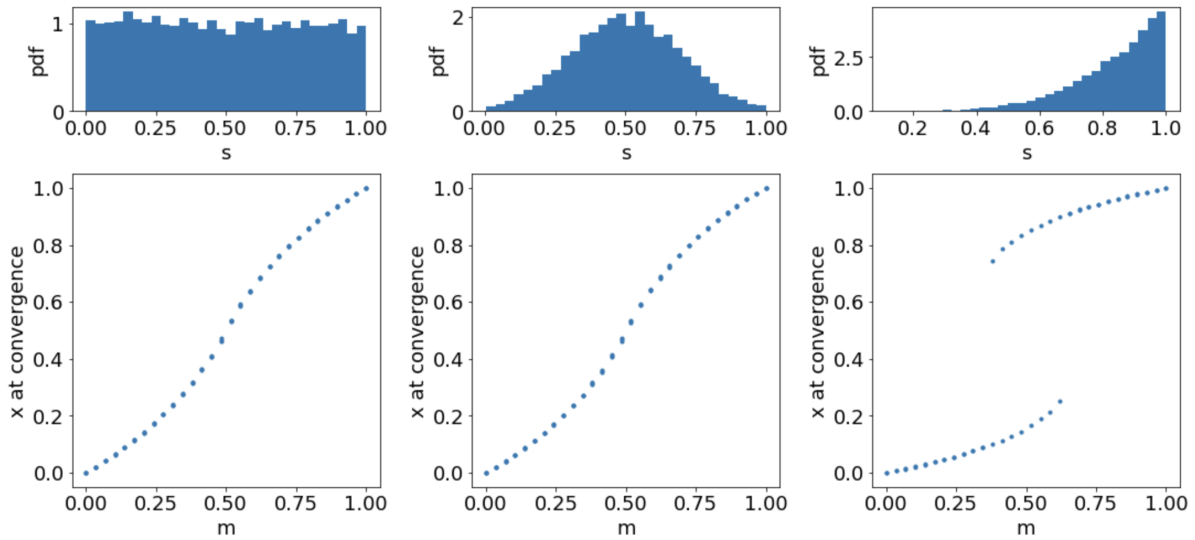

**Figure S2.** Result of the simulations assuming each individual is on the gradient of individual to social learners. The distributions of  $s$ , which indicate the degree of social learning of each individual, are shown on the top panels. The corresponding results of  $x$  at convergence as a function of  $m$  are shown on the bottom panels. Left column: uniform distribution  $s$ . Middle column: truncated normal distribution  $s$ , with mean 0.5 and standard deviation 0.2, truncated to between 0 and 1. Right column: Beta distribution  $s$ , with shape parameters  $a = 5$ ,  $b = 1$ . All simulations involve 10,000 individuals,  $\alpha = 1.5$ .

The model in the main text makes the parsimonious dichotomy of social vs. individual learners. In reality, one would expect each individual to be on a spectrum between pure individual and pure social learning.

Here we present a model with this modification and show the major conclusions of the baseline model presented in the main text do not change.

Consider the individual  $i$  favoring  $Y$ , the transition probability of them changing to  $X$  is:

$$P_i(Y \rightarrow X) = (1 - s_i)m + s_i f(x), \quad (\text{S8})$$

where  $s_i$  is a parameter between 0 and 1. It characterizes the degree of social learning of the individual  $i$ , through weighting the merit of the options and the conformity response,  $f(x)$ . The extreme value  $s_i = 1$  denotes fully social learner, and  $s_i = 0$  denotes fully individual learner. The other variables are defined as the same as the main text. Similarly, the transition probability from  $X$  to  $Y$  is:

$$P_i(X \rightarrow Y) = (1 - s_i)(1 - m) + s_i f(1 - x), \quad (\text{S9})$$

We computationally simulate a distribution of  $s_i$  and run the system to equilibrium. The results for uniform, normal, and right-skewed distributions  $s_i$  are shown in Fig. S2. For both uniformly and normally distributed  $s$ , there is a smooth increase of  $x$  with  $m$ , and only one fixed point appears for each set of parameters. This behavior is similar to the original model with  $s < s_c$ . For a right-skewed distribution of  $s$  (more social learning), a bi-stable region of  $x$  occurs for mid-range  $m$ , which is similar to the behavior of the original system with  $s > s_c$  (Fig. 2(D) of main text).

## 5.2 Spatial extension

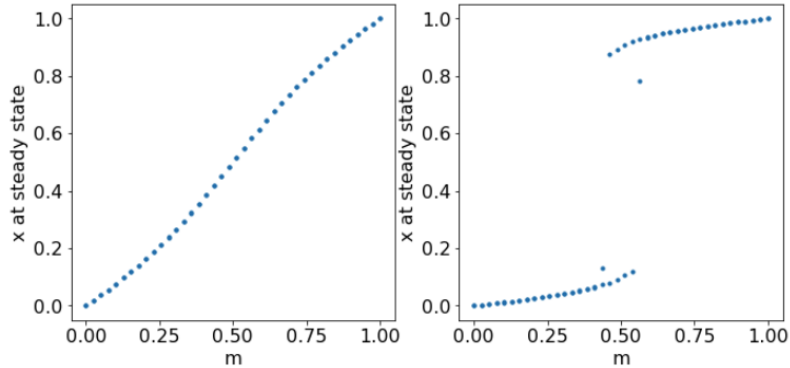

**Figure S3.** Proportion of individuals favoring option  $X$  at steady state for the 2D grid model. Left: small  $s$ ,  $s = 0.5$ . Right: large  $s$ ,  $s = 0.95$ . Both simulations involve 4000 individuals in a 200 by 200 grid, and  $\alpha = 1.8$ .

We consider the spatial extension of the model presented in the main text, which assumes a well-mixed population. We consider individuals arranged on a 2-D lattice. A proportion  $s$  of those individuals are randomly assigned to be social learners, and  $1 - s$  individual learners. In each time step, the individual learners' transition probability from  $X$  to  $Y$  is  $P(X \rightarrow Y) = m$ , and that from  $Y$  to  $X$  is  $P(Y \rightarrow X) = 1 - m$ . Social learners' opinion transitions are affected by the opinion of their four neighbors.  $P(X \rightarrow Y) = f(x_n)$ , where  $x_n$  is the portion of neighbors favoring  $X$ . We determine the convergence of simulations through the following process. We take the last  $w$  steps of the time series for  $x$ , the proportion favoring option  $X$ , and compute the standard deviation that time series. When the standard deviation is smaller than a critical threshold, we determine the simulation has converged. In this simulation, the window size  $w = 30$ , and the critical threshold is 0.05. Also, we ensured the time series requires a minimum length of 40 iterations for it to converge.

Examples of the simulation results, with periodic boundary conditions, are shown in Fig. S3. Bistable states appear for large  $s$ , similar to Fig. 2(D) of the main text.

### 5.3 Noise extension

In this extension, we study the baseline model under the presence of noise using simulations. We consider  $N$  individuals, where each individuals' transition rates in each time step are the same as that in the baseline model,  $P(Y \rightarrow X) = m$  for individual learners, and  $P(Y \rightarrow X) = f(x)$  for social learners. Noise is added to the system as follows. In each time step, after updating according to the assigned transition rates, each individual has some probability of replacing their chosen option by a random one between  $X$  and  $Y$ . We refer to this probability as the noise level. For example, 5% noise means each individual has a 5% probability of adopting a random option in each time step.

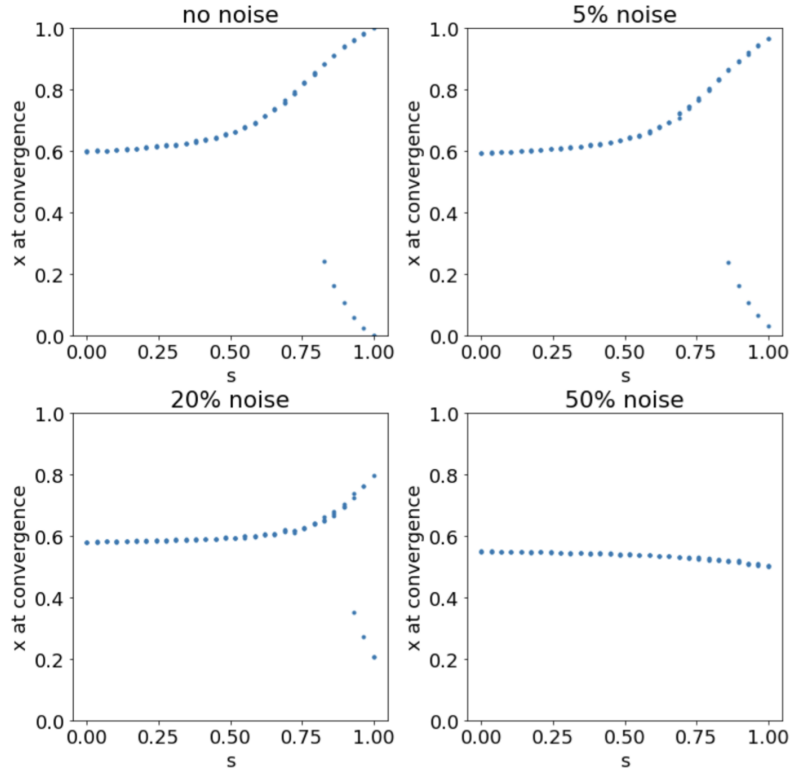

**Figure S4.** Proportion of individuals favoring option  $X$  at steady state (noise extension model). The parameters of the simulation are  $m = 0.6$  and  $\alpha = 1.5$ , the same as those of Fig. 2(B) of the main text.

We simulate this extension with the same parameters as Fig. 2(B) of the main text with the presence of varying levels of noise, and the results are shown in Fig. S4. We find that in the presence of a small amount of noise, the model reaches similar results. As the noise level increases,  $x$  at convergence drifts closer to 0.5. When the level of noise is large, the bifurcation behavior disappears (such as the 50% noise panel in Fig. S4). This is expected because the nature of the noise biases the system towards a 50–50 split between the two options.

### 5.4 Opinion strength extension

We formulate an extension of our model to account for the strength of opinions about options motivated by the model of Couzin et al. [20]. The model in Couzin et al. assumes two types of individuals, informed

and uninformed. Each informed person  $i$  has a preferred state between  $X$  and  $Y$ , and if one is in their preferred state, there is probability  $w_i$ , the strength of the opinion, that they stay in the original state. With probability  $1 - w_i$ , they take a sample of the population and change their opinion to align with the majority of the sample. This conformity response follows an s-shape. The uninformed have strength 0.

In this extension, we extend the transition rates of the individual learners from  $X$  to  $Y$  as,  $P_{XY}^{(i)} = (1 - w_x)(1 - m)$ , where  $w_x$ , a parameter taking on values between 0 and 1, is the relative strength of opinion about  $X$  compared to that about  $Y$ . This modification denotes that there is probability  $w_x$  that a person holding opinion  $X$  stays in this opinion, regardless of merit. Similarly, the transition rates of individual learners from  $Y$  to  $X$  is  $P_{YX}^{(i)} = w_x m$ . The transition rates of the social learners and the other dynamics of the system remain the same. In this formulation, the individual learners in our model are similar to the informed individuals in Couzin et al., and the social learners are similar to the uninformed individuals in Couzin et al.

Panel A of Fig. 3 in the main text is to show that the extended model recovers the results of the baseline model in the case of both  $X$  and  $Y$  held at equal strength ( $w_x = 0.5$ ). Since the parameters  $m$  and  $\alpha$  used are the same as that in Fig. 2(B) of our main text, we expect Fig. 3(A) to show similar behavior with that of Fig. 2(B), and it is indeed the case. In Fig. 3(B), we simulate the case where the high-merit option ( $X$ ) is held at weaker strength ( $w_x = 0.3$ ) than the low-merit option ( $Y$ ). This scenario is to be compared with Fig. 2(B) in Couzin et al. [20]. In both our simulation and Couzin et al., the two branches of the bifurcation are flipped compared to that of Fig. 3(A) of our main text. In the case of social learners under a critical threshold, the majority favors the low-merit option, and when the proportion of social learners exceed the threshold, the outcome of the majority favoring the high-merit option becomes possible.

## 6 Code availability

The code used in this manuscript to analyze the baseline model and the extensions in SI 5.1–5.4 is available at [https://github.com/vc-yang/social\\_learners\\_collective\\_decision](https://github.com/vc-yang/social_learners_collective_decision).

## References

1. Claidière, N. & Whiten, A. Integrating the study of conformity and culture in humans and nonhuman animals. *Psychol. Bull.* **138**, 126 (2012).
2. Asch, S. E. Effects of group pressure upon the modification and distortion of judgments. *Organ. Infl. Process.* 295–303 (1951).
3. Hoppitt, W. & Laland, K. N. *Social Learning: An Introduction to Mechanisms, Methods, and Models* (Princeton University Press, 2013).
4. Meder, B., Le Lec, F. & Osman, M. Decision making in uncertain times: What can cognitive and decision sciences say about or learn from economic crises? *Trends Cogn. Sci.* **17**, 257–260 (2013).
5. Spiegelhalter, D. J. & Riesch, H. Don't know, can't know: Embracing deeper uncertainties when analysing risks. *Philos. Transactions Royal Soc. A: Math. Phys. Eng. Sci.* **369**, 4730–4750 (2011).
6. Campbell, A., Converse, P. E., Miller, W. E. & Stokes, D. E. *The American Voter* (University of Chicago Press, 1980).

7. Lo, A. W. & Mueller, M. T. Warning: Physics envy may be hazardous to your wealth! *J. Invest. Manag. (JOIM)* **8** (2010).
8. Han, P. K., Klein, W. M. & Arora, N. K. Varieties of uncertainty in health care: A conceptual taxonomy. *Med. Decis. Mak.* **31**, 828–838 (2011).
9. Galesic, M., Kause, A. & Gaissmaier, W. A sampling framework for uncertainty in individual environmental decisions. *Top. Cogn. Sci.* **8**, 242–258 (2016).
10. Boyd, R. & Richerson, P. J. *Culture and the Evolutionary Process* (University of Chicago press, 1988).
11. Young, H. P. The evolution of conventions. *Econom. J. Econom. Soc.* 57–84 (1993).
12. Salganik, M. J., Dodds, P. S. & Watts, D. J. Experimental study of inequality and unpredictability in an artificial cultural market. *Science* **311**, 854–856 (2006).
13. Centola, D. The spread of behavior in an online social network experiment. *Science* **329**, 1194–1197 (2010).
14. Morgan, T. J. H. & Laland, K. N. The biological bases of conformity. *Front. Neurosci.* **6**, 87 (2012).
15. Claidiere, N., Bowler, M. & Whiten, A. Evidence for weak or linear conformity but not for hyper-conformity in an everyday social learning context. *PLoS ONE* **7** (2012).
16. Latané, B. The psychology of social impact. *Am. Psychol.* **36**, 343 (1981).
17. Claidière, N., Bowler, M., Brookes, S., Brown, R. & Whiten, A. Frequency of behavior witnessed and conformity in an everyday social context. *PloS ONE* **9** (2014).
18. Morgan, T., Rendell, L., Ehn, M., Hoppitt, W. & Laland, K. The evolutionary basis of human social learning. *Proc. Royal Soc. B: Biol. Sci.* **279**, 653–662 (2012).
19. Strogatz, S. H. *Nonlinear dynamics and chaos* (CRC press, 2018).
20. Couzin, I. D. *et al.* Uninformed individuals promote democratic consensus in animal groups. *Science* **334**, 1578–1580 (2011).
